# Supplementary material for: A Distributed, Decoupled System for Losslessly Streaming Dynamic Light Probes to Thin Clients
Source: arXiv:2103.05875 source file (2021-03-10)
Supplement: Supplementary file 1 [file supplemental.tex]

\section{Server-side Rendering (Algorithm 1)}

\begin{algorithm}
    \SetAlgoLined
    ray trace probe textures\;
    \For{each client}{
        bind permanent client probe textures\;
        clear and bind probe update textures\;
        clear and bind probe index buffer\;
        \tcp{1st pass on GPU}
        calculate probe indices in client view\;
        \For{each probe in client view}{
            \If{probe info has changed and active}{
                update probe info in client probe textures\;
                append probe info to probe update textures\;
                append probe to probe index buffer\;
            }
        }
        \tcp{2nd pass on GPU}
        compress probe update textures\;
        \tcp{cpu}
        download and send probe index buffer and probe update textures\;
    }
\caption{Selective probe update on server}
\end{algorithm}

\section{Selective Probe Update (Algorithm 2)}
\begin{algorithm}
    \SetAlgoLined
    \tcp{on CPU}
    receive probe indices\;
    receive compressed probe update textures\;
    upload data to GPU\;
    \tcp{on GPU}
    decompress probe update textures\;
    update probe textures from probe update textures and indices\;
\caption{Probe update on client}
\end{algorithm}
\vspace{-0.5cm}

\section{Probe Atlas Arrangement}
As each texel represents directional information it is obvious that adjacent probes contain angular redundancy. We have tested different texel arrangements for the probe atlas. The original DDGI paper uses 10x10 pixels for the core probe color information (Figure~\ref{fig:probeatlasarrangement}, left). We rearrange texels from four probes in a 2x2 block (Figure~\ref{fig:probeatlasarrangement}, center) and from eight probes in a 4x4 block (Figure~\ref{fig:probeatlasarrangement}, right) so that texels of neighboring probes but with similar directions during probe tracing are adjacent in the probe atlas. This way adjacent pixels often contain similar values which support algorithms such as Run Length Encoding (RLE) or Delta Encoding. However, our analysis reveals that the lossless HEVC video encoder could exploit redundancy best in the original layout where individual probes are arranged as individual blocks. This result holds for lossless as well as for lossy compression (see compressed sizes in Figure~\ref{fig:probeatlasarrangement}). HEVC compression works on texel blocks which can be quite similar for multiple probes across the probe atlas with respect to different compression metrics. The video encoder therefore has a better chance in exploiting redundancies across \textit{all} probes in a volume than from just angular probe redundancy of \textit{neighboring} probes.

\begin{figure*}[t]
\setlength\tabcolsep{2pt}%
\begin{tabularx}{\textwidth}{ccc}
   \includegraphics[ width=0.33\linewidth, keepaspectratio]{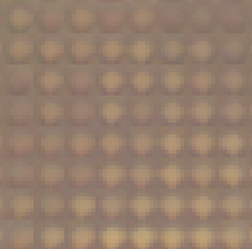} &
   \includegraphics[ width=0.33\linewidth, keepaspectratio]{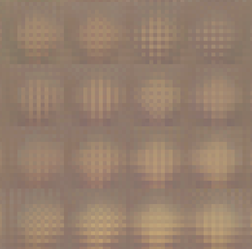} &
   \includegraphics[ width=0.33\linewidth, keepaspectratio]{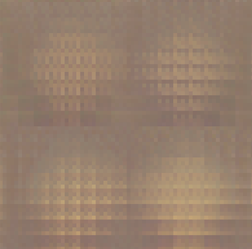}\\
 \textsc{1x1 Probe Block Layout} & \textsc{2x2 Interleaved Texel Layout} & \textsc{4x4 Interleaved Texel Layout}\\
\end{tabularx}
\caption{\textbf{Probe Atlas Arrangement Analysis.}~\normalfont Probe atlas sizes are given for \textsc{Greek Villa} scene averaged for 278 frames: (left) 1x1 probe, original DDGI arrangement: 224 kilobytes, (center) 2x2 probes interleaved: 238 kilobytes, (right) 4x4 probes interleaved: 250 kilobytes.}
\label{fig:probeatlasarrangement}
\end{figure*}

\section{Network Throughput}

We show the consumed bandwidth over time using our different bandwidth reduction methods (Figure~\ref{fig:bandwidthtomb}-\ref{fig:bandwidthnightstreet}).
\begin{itemize}
    \item \textit{Uncompressed}: direct uncompressed texture transfer, Section 3.2
    \item \textit{Encoded}: full texture compression, Section 3.3
    \item \textit{Culling}: update only probes in client view, send full atlas, Section 3.4
    \item \textit{Culling, Packing, No caching}: update only probes in client view, reduce atlas to active and updates probes, no cache for previously updated probes, Section 3.4
    \item \textit{Packing and Caching}: as before but previously transmitted probe indices are cached for probe placement in atlas to increase temporal stability of probe textures, Section 3.4
\end{itemize}

\begin{table}[t]
\small
\begin{tabularx}{\columnwidth}{p{0.2\columnwidth}ccc}
\hline
$T_{Render}$ & \textsc{Tomb Buddha} & \textsc{Greek Villa} & \textsc{Night Street}\\
\hline
Mean (ms)         & \textbf{3.49}      & \textbf{6.39}     & \textbf{3.57}  \\
Std. Dev. (ms)    & 0.34      & 0.46     & 0.34  \\
Min (ms)          & 2.36      & 5.50     & 3.15  \\
Max (ms)          & 6.48      & 7.38     & 5.54   \\
\hline
\end{tabularx}
\vspace{0.1cm}
\caption{\textbf{Client render times.}~\normalfont Timings evaluated on gaming GPU (NVIDIA RTX 2080 Ti).}
\label{table:clientrenderanalysisperscene}
\end{table}

\begin{figure}[h]
\includegraphics[width=\linewidth, trim=0 0.7cm 0 0.5cm, clip]{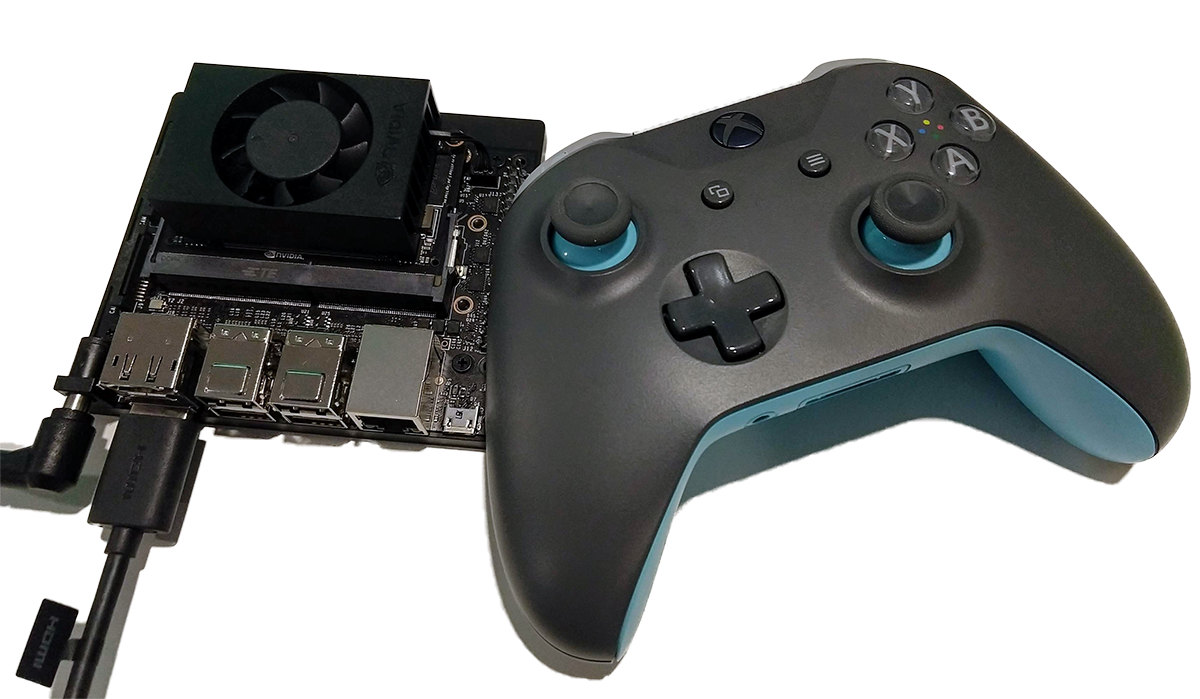}
\caption{\textbf{Thin Client : NVIDIA Xavier NX.}~\normalfont
The portable Tegra GPU on the NVIDIA Xavier NX developer board provides two low-power hardware units for accelerated HEVC video decoding. Timings for decoding are given in Table 3 in the paper.}
\label{fig:xaviernx}
\vspace{-3mm}
\end{figure}

\section{Selective Probe Transmission}
We discuss our recommended strategy for selective probe transmission in Section 3.4 in the paper. Our method computes all probes shading points visible in the client's camera view frustum and then augments that set with an estimate of all probes shading points visible from the camera's current position. This is computed on the server by rasterizing the client's primary view and then tracing 1024 rays uniformly distributed on a sphere centered at the camera position. The raster pass and ray tracing pass combined yield a set of world space positions. All probes that shade these positions are then marked for transmission.

To further evaluate our selection mechanism, note that only probes that have changed texel values since they were last transmitted could possibly convey useful information to the client. Therefore, the number of changed probes is an upper bound on the number of probes that should ever be sent. From the other direction, all probes that have new data and shade points in the client's primary view frustum \emph{must} be sent to correctly render the current view on the client. The number of these probes is the lower bound on the number of probes sent. As shown in Figure~\ref{fig:cullingschemes}, our selection mechanisms achieves the image quality of the higher bound while transmitting a number of probes closer to the lower bound. Further, the number of rays used to gather potentially visible points around the camera can be adjusted depending on the constraints of image quality vs. bandwidth.

\newpage

\begin{figure}[ht]
    \includegraphics[width=\linewidth]{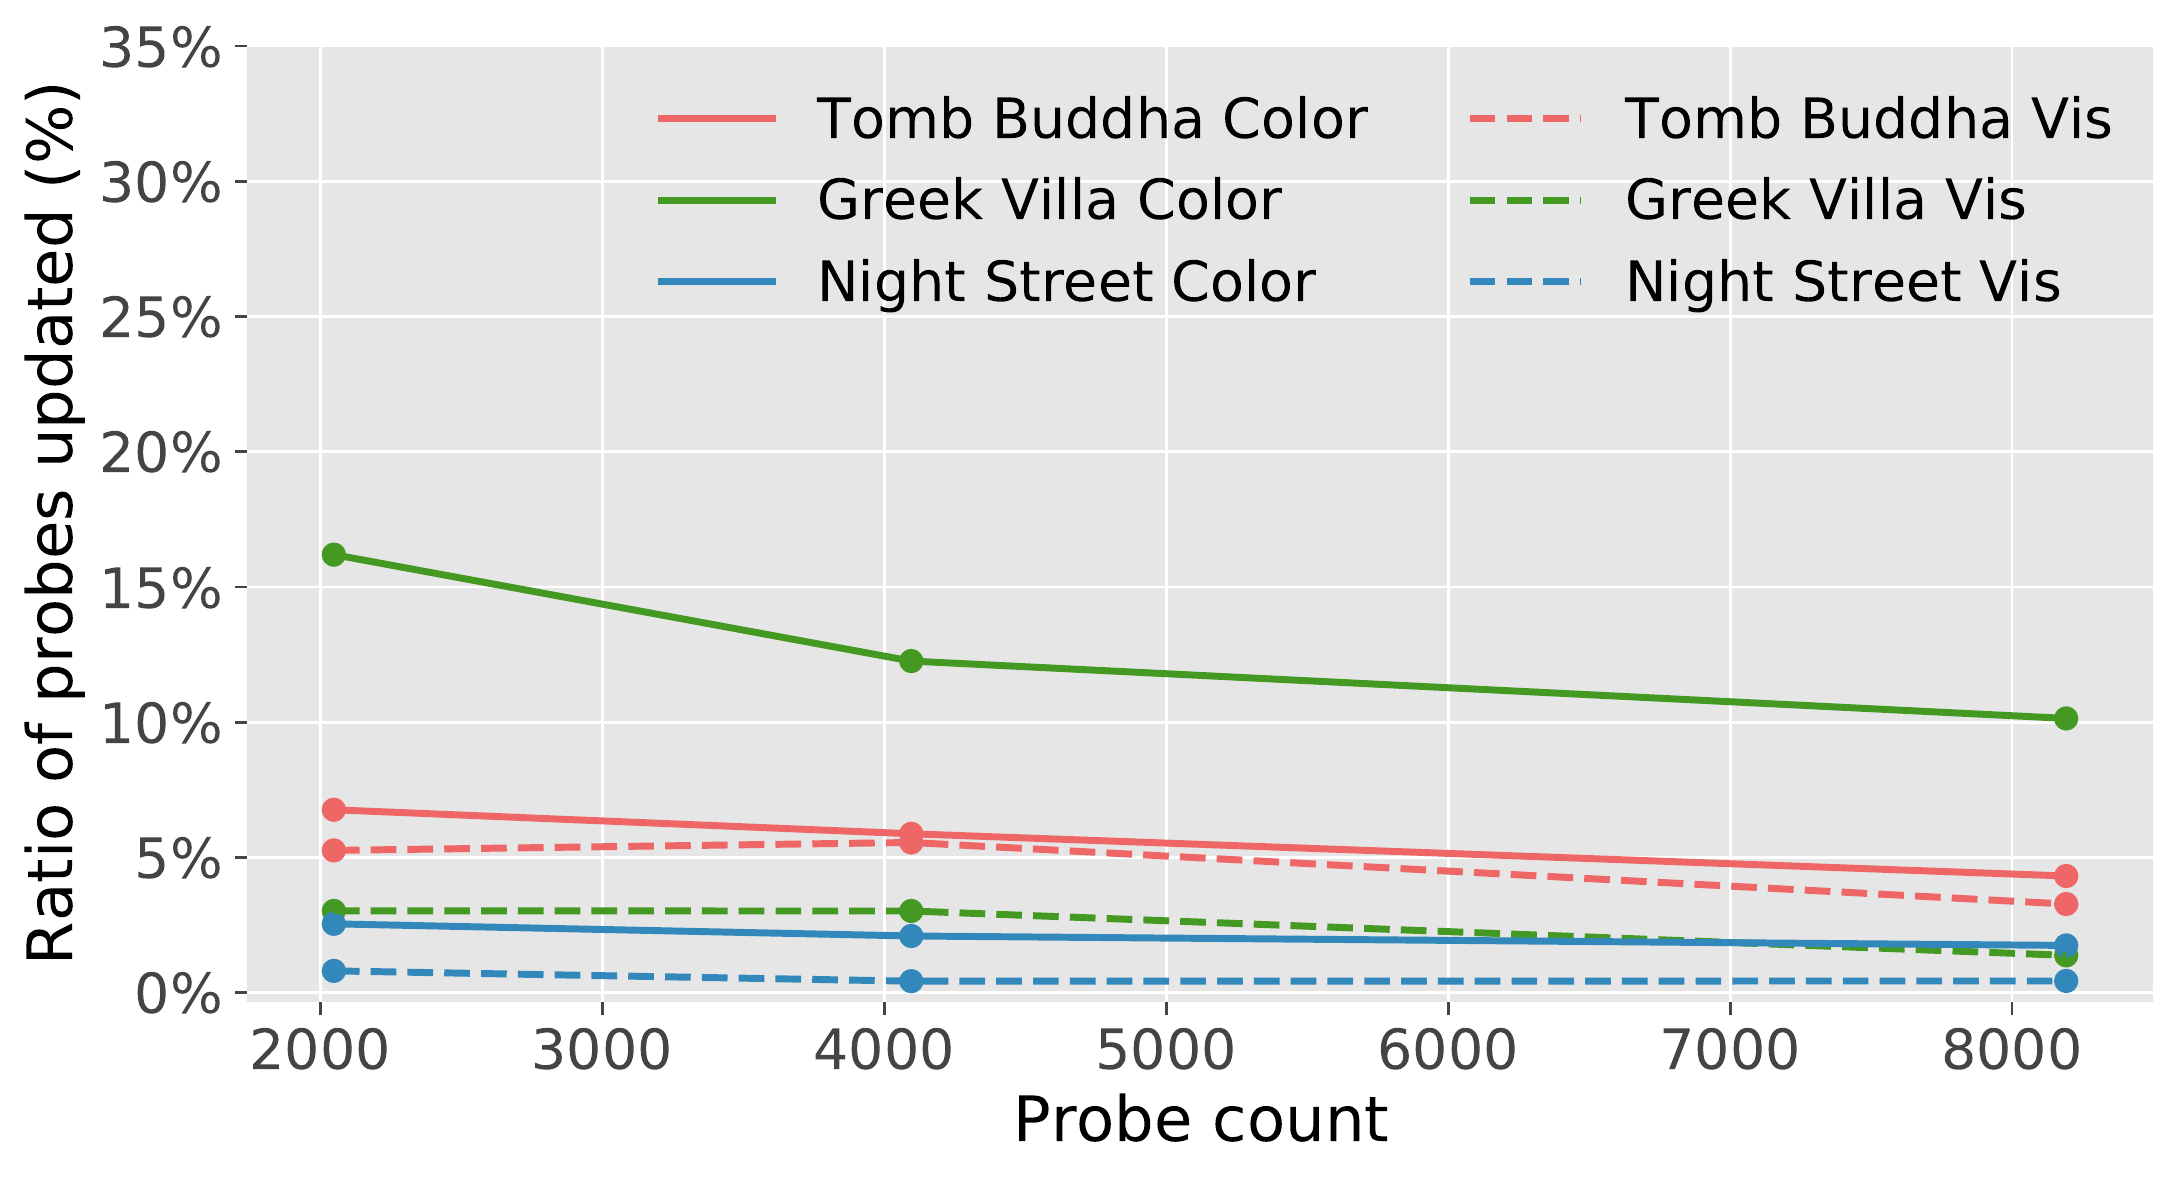}\\
    \includegraphics[width=\linewidth]{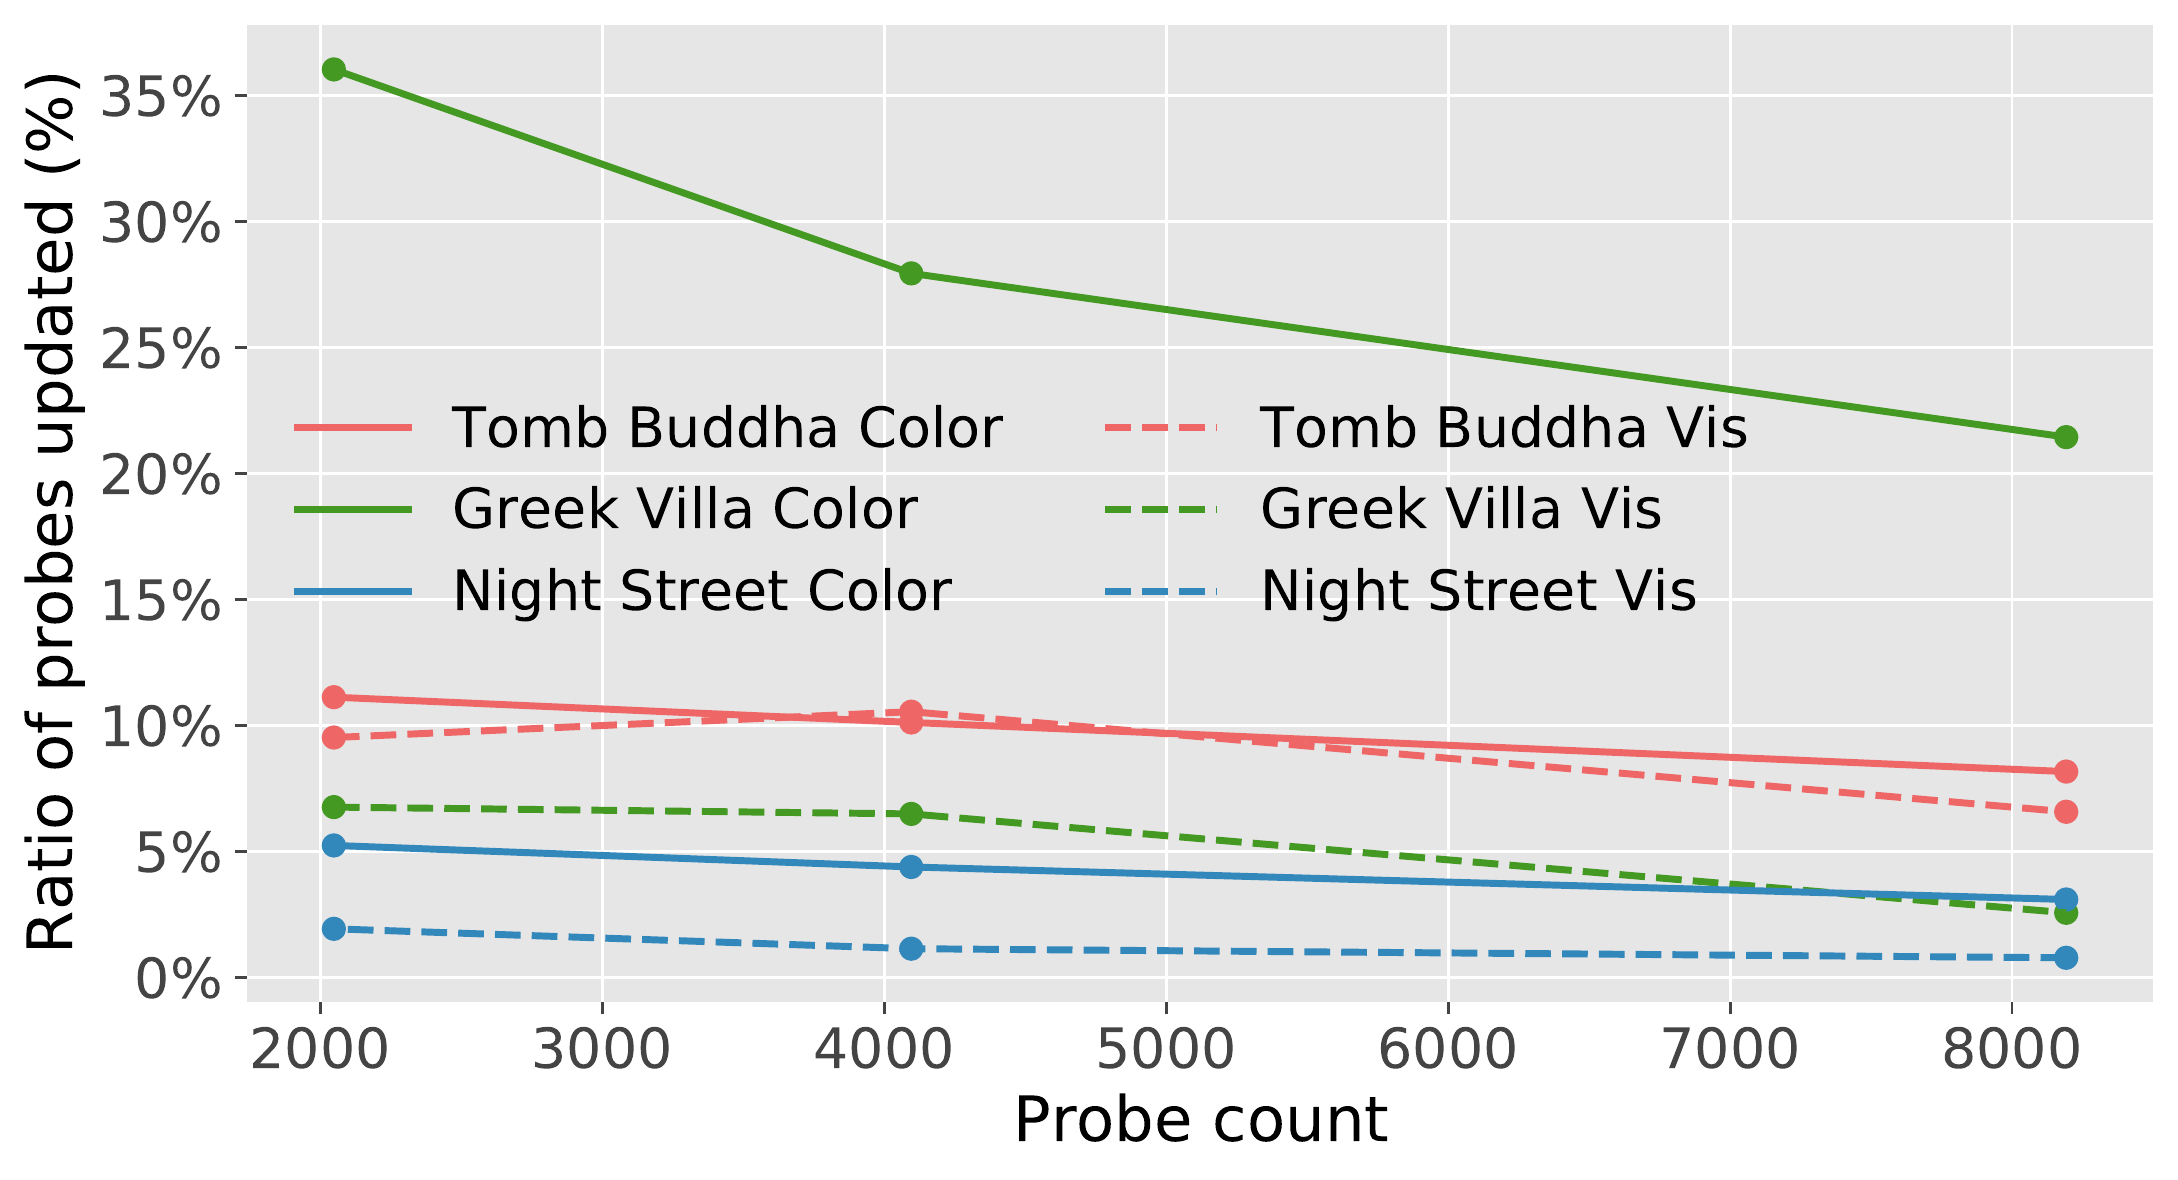}\\
    \includegraphics[width=\linewidth]{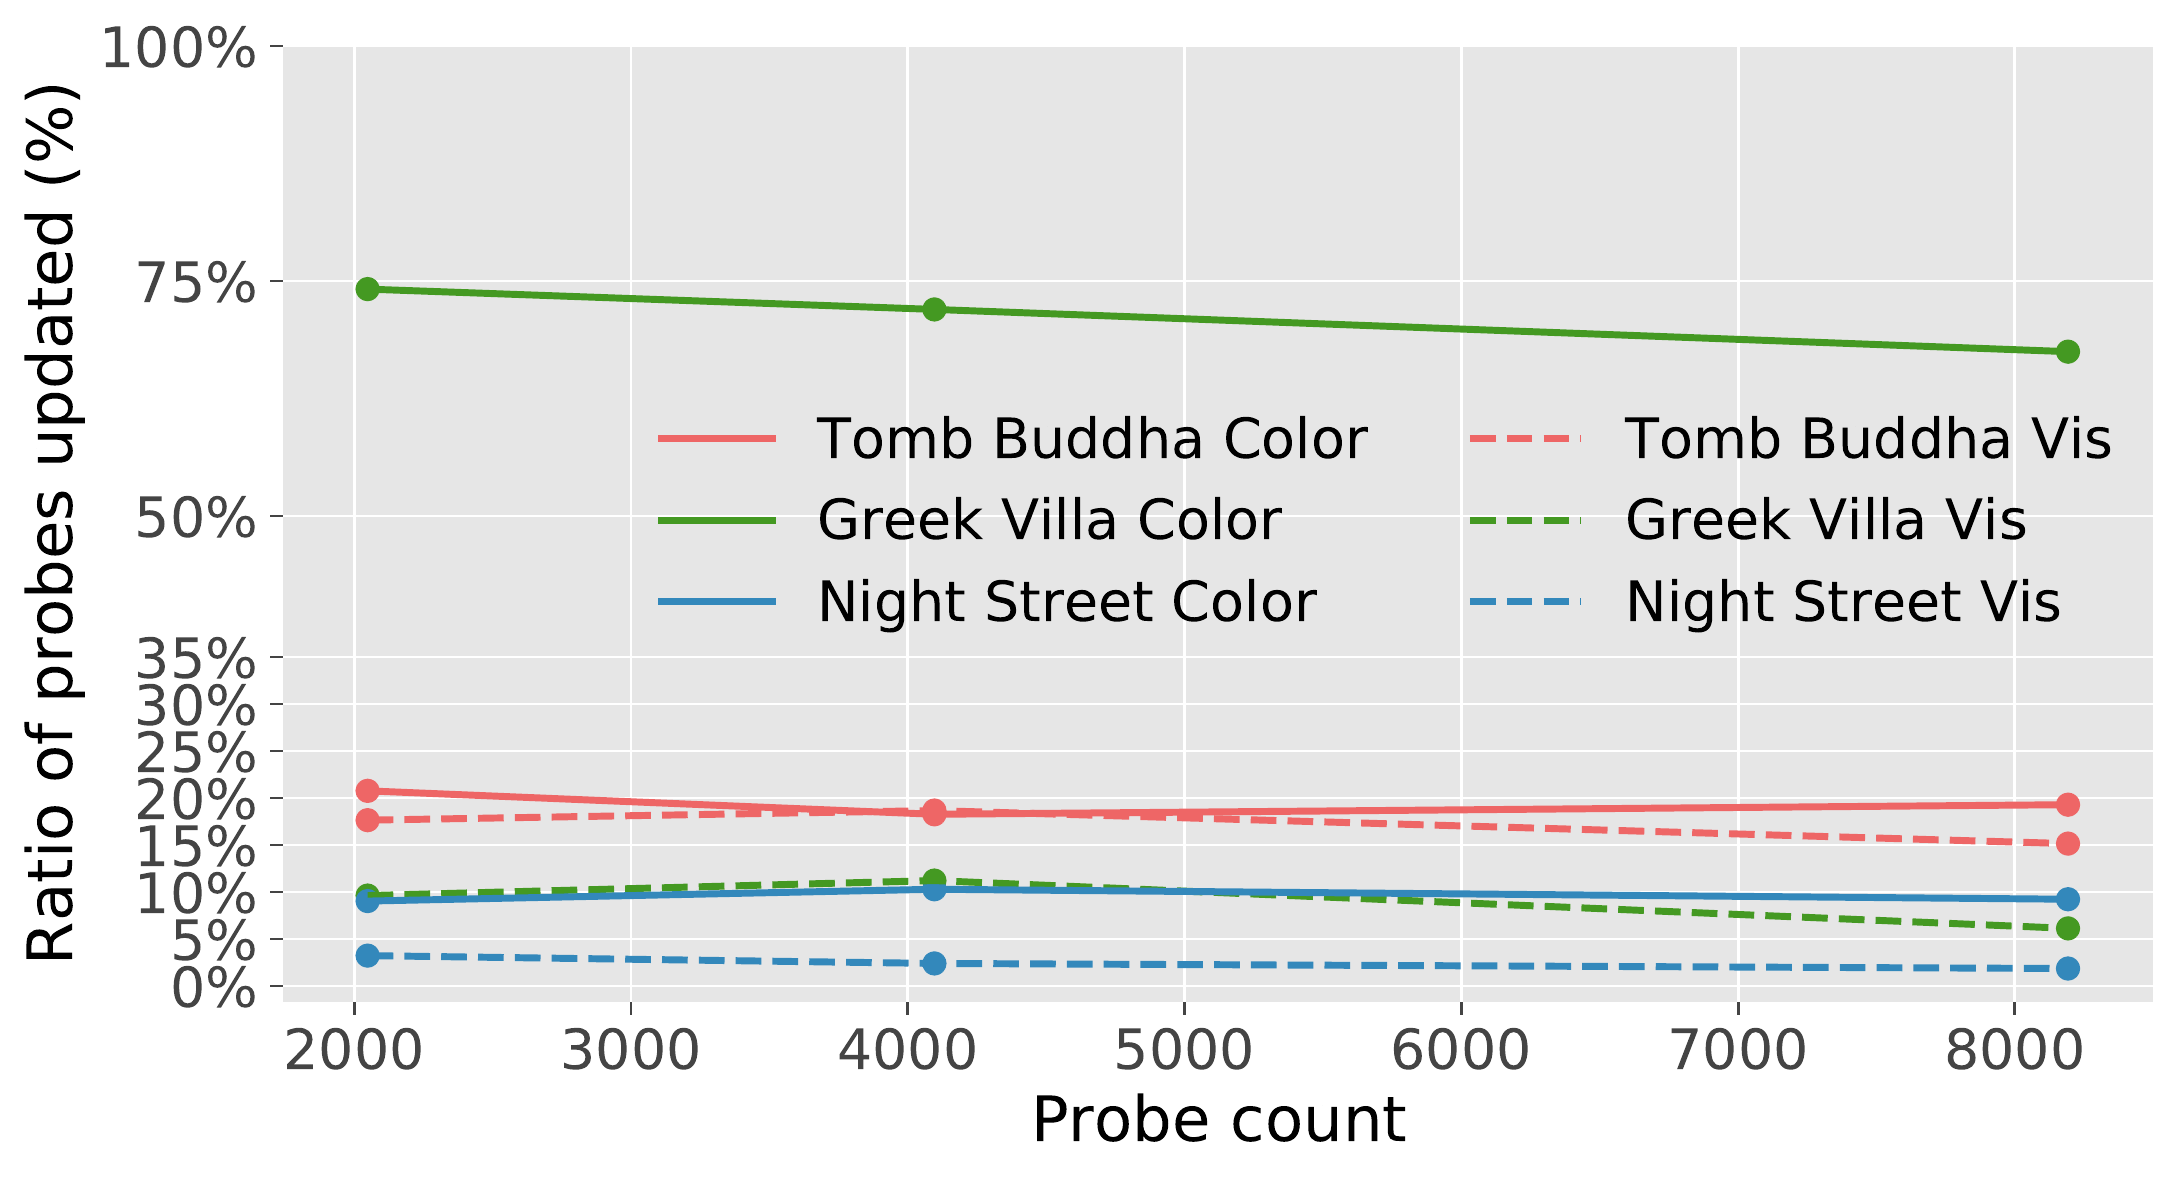}
    \caption{\textbf{Selective Probe Reduction Performance.}~ \normalfont  Average percentage of probes updated (over time) with unchanged probes removed. The most aggressive culling transmits probes within the primary view only (top), but suffers from artifacts (see Figure 3). Our recommended method transmits more probes by augmenting the primary view set with a potentially visible set of probes from the camera's perspective (middle). This approach gives the same image as doing no selection but sends significantly fewer probes than transmission without probe selection (bottom).}
    \label{fig:SelectiveProbeUpdatePerformance}
\end{figure}

\begin{figure*}[t]
\setlength\tabcolsep{2pt}%
\begin{tabularx}{\textwidth}{cc}
   \includegraphics[ width=0.5\linewidth, keepaspectratio]{figures/culling/ClientReference.png} &
   \includegraphics[ width=0.5\linewidth, keepaspectratio]{figures/culling/ClientCullOutsidePrimaryView.jpg}\\
 \textsc{Client reference view} & \textsc{Primary view probes only (1261 probes sent)}\\
    \includegraphics[ width=0.5\linewidth, keepaspectratio]{figures/culling/ClientNoCull.jpg} &
   \includegraphics[ width=0.5\linewidth, keepaspectratio]{figures/culling/ClientGatherPotentiallyVisible.jpg}\\
 \textsc{All changed probes (3299 probes sent)} & \textsc{Potentially visible probe set (1710 probes sent)}\\
\end{tabularx}
\caption{\textbf{Selective Probe Transmission.}~\normalfont 
Our Greek Villa scene with 4096 probes. Probe selection is done relative to a client reference view known to the server (top left). Sending only probes within the client primary view gives large outdated regions (top right, outdated regions rendered in black). In this case, 1261 probes are transmitted. All regions are up to date when all active probes are sent (bottom left). In this case, 3299 probes are transmitted. Finally, the same image quality is achieved with our potentially visible probe set estimation (bottom right). In this case, though the image is the same, only 1710 probes are transmitted.}
\label{fig:cullingschemes}
\end{figure*}

\newpage

%% %%%%%%%%%%%%%%%%%%%%%%%%%%%%%%%%%%%%%%%%%%%%%%%%%%%%%%%%%%%%%%%%%%%%%%%%%%%%%%%%%%%%%%%%%%%%%%%%%%%%%%%
% Greek Villa
%% %%%%%%%%%%%%%%%%%%%%%%%%%%%%%%%%%%%%%%%%%%%%%%%%%%%%%%%%%%%%%%%%%%%%%%%%%%%%%%%%%%%%%%%%%%%%%%%%%%%%%%%

\begin{figure*}[t]
\setlength\tabcolsep{2pt}%
\begin{tabularx}{\textwidth}{c}
   \includegraphics[ width=\linewidth, keepaspectratio]{figures/results_timeplots_latency_size/Latency_greek_villa_30_10_cache_cull_indirect_2.pdf}\\
   \includegraphics[ width=\linewidth, keepaspectratio]{figures/results_timeplots_latency_size/Size_greek_villa_30_10_cache_cull_indirect_2.pdf}\\
\end{tabularx}
\begin{tabularx}{\textwidth}{p{0.15\textwidth}p{0.25\textwidth}p{0.18\textwidth}p{0.20\textwidth}l}
\hline
Streaming Data & Average Latency (Std.Dev.) &  Min/Max Latency & Average Size (Std.Dev.) & Min/Max Size\\
\hline
Irradiance & 37.01 ms (20.361) & 10 ms / 196 ms & 10.52 kB (4.06) & 3.02 kB / 33.941 kB \\
Visibility & 39.03 ms (20.339) & 8 ms / 255 ms & 0.692 kB (4.951) & 0.09 kB / 97.680 kB \\
\hline
\end{tabularx}
\caption{\textbf{Detail time series plot for scene \textsc{Greek Villa} with view culling.}~\normalfont During recording the client moves around in the scene. The lighting in the scene permanently changes due to a fast day-night cycle. Probe visibility is only updated when the user can see the orrery in the scene (around times 0:18 and 0:40) reducing the amount of demanding transfers. Streaming settings: 30 Hz irradiance update rate, 10 Hz visibility update rate, selective probe updates for enabled, delta-encoded index buffer probe index buffer with caching, client view culling enabled.}
\label{fig:timeplot_greekvilla_culling}
\end{figure*}

\begin{figure*}[t]
\setlength\tabcolsep{2pt}%
\begin{tabularx}{\textwidth}{c}
   \includegraphics[ width=\linewidth, keepaspectratio]{figures/results_timeplots_latency_size/Latency_greek_villa_30_10_cache_no_cull_2.pdf}\\
   \includegraphics[ width=\linewidth, keepaspectratio]{figures/results_timeplots_latency_size/Size_greek_villa_30_10_cache_no_cull_2.pdf}\\
\end{tabularx}
\begin{tabularx}{\textwidth}{p{0.15\textwidth}p{0.25\textwidth}p{0.18\textwidth}p{0.20\textwidth}l}
\hline
Streaming Data & Average Latency (Std.Dev.) &  Min/Max Latency & Average Size (Std.Dev.) & Min/Max Size\\
\hline
Irradiance & 53.31 ms (28.163) & 13 ms / 234 ms & 57.95 kB (16.178) & 15.53 kB / 149.87 kB \\
Visibility & 45.57 ms (29.33) & 9 ms / 229 ms & 5.67 kB (14.537) & 0.09 kB / 69.62 kB \\
\hline
\end{tabularx}
\caption{\textbf{Detail time series plot for scene \textsc{Greek Villa} without view culling.}~\normalfont The scene is the same as in the previous plot with the difference that in this plot all changing probes are transferred to the client. The degree of lighting change for the day-night cycle can easily be observed in the cycle of the resulting encoded texture size. Probe visibility is updated whenever the orrery changes position (time 0:20 to 1:15). Streaming settings: 30 Hz irradiance update rate, 10 Hz visibility update rate, selective probe updates for enabled, delta-encoded index buffer probe index buffer with caching, client view culling disabled.}
\label{fig:timeplot_greekvilla_noculling}
\end{figure*}

\begin{figure*}[ht]
\centering
\includegraphics[width=0.9\textwidth]{figures/results_timeplots/bandwidth_greekvilla_w_uncompressed.pdf}
\caption{\textbf{Method overview showing consumed network bandwidth for scene \textsc{Greek Villa}.} The overview shows that our probe reduction and compression method reduces the required network traffic but at least one order of magnitude.}
\label{fig:bandwidthgreekvillawithuncompressed}
\end{figure*}

\begin{figure*}[ht]
\centering
\includegraphics[width=0.9\textwidth]{figures/results_timeplots/bandwidth_greekvilla_.pdf}
\caption{\textbf{Method overview (excluding uncompressed transfer) showing consumed network bandwidth for scene \textsc{Greek Villa}.}~\normalfont During recording the client moves on a fixed animation path through the scene. The probe volume update rate has a strong but sub-linear influence on the consumed network bandwidth and can be seen as a 'quality knob' controlling the dynamic quality of global illumination (GI) for the client. Furthermore, our probe selection and caching schemes significantly reduce the amount of transferred data. Probe selection alone \textit{without} caching can actually increase the amount of transferred data as encoding efficiency is decreased. Probe selection in combination with index caching however optimizes for efficient temporal encoding of only changed probes resulting in a significant reduction of bandwidth compared to full volume encoding. The culling method can be tuned for even more aggressive probe reduction if the client field of view is limited further (Fig.~\ref{fig:cullingschemes}, not shown here) but can result in perceivable artifacts as the the probe update is delayed after quick turns of client. }
\label{fig:bandwidthgreekvilla}
\end{figure*}

%% %%%%%%%%%%%%%%%%%%%%%%%%%%%%%%%%%%%%%%%%%%%%%%%%%%%%%%%%%%%%%%%%%%%%%%%%%%%%%%%%%%%%%%%%%%%%%%%%%%%%%%%
% Night Street
%% %%%%%%%%%%%%%%%%%%%%%%%%%%%%%%%%%%%%%%%%%%%%%%%%%%%%%%%%%%%%%%%%%%%%%%%%%%%%%%%%%%%%%%%%%%%%%%%%%%%%%%%

\begin{figure*}[t]
\setlength\tabcolsep{2pt}%
\begin{tabularx}{\textwidth}{c}
   \includegraphics[ width=\linewidth, keepaspectratio]{figures/results_timeplots_latency_size/Latency_night_city_30_10_cache_cull_indirect.pdf}\\
   \includegraphics[ width=\linewidth, keepaspectratio]{figures/results_timeplots_latency_size/Size_night_city_30_10_cache_cull_indirect.pdf}\\
\end{tabularx}
\begin{tabularx}{\textwidth}{p{0.15\textwidth}p{0.25\textwidth}p{0.18\textwidth}p{0.20\textwidth}l}
\hline
Streaming Data & Average Latency (Std.Dev.) &  Min/Max Latency & Average Size (Std.Dev.) & Min/Max Size\\
\hline
Irradiance & 35.21 ms (13.813) & 16 ms / 161 ms & 1.02 kB (1.373) & 0.04 kB / 24.15 kB \\
Visibility & 30.76 ms (17.406) & 11 ms / 154 ms & 2.02 kB (3.573) & 0.15 kB / 52.45 kB \\
\hline
\end{tabularx}
\caption{\textbf{Detail time series plot for scene \textsc{Night Street} with view culling.}~\normalfont During recording the client moves around in the city scene. The lighting in the scene permanently changes locally for moving cars on the street and for a rotating emergency light. Probe visibility is only updated when the user can see the moving cars which happens frequently for some probes during the time of recording. Although the scene contains 8000 probes the transmitted data the probe selection and encoding is surprisingly efficient as at a point in time only a limited number of probes contribute to the view of the client. Streaming settings: 30 Hz irradiance update rate, 10 Hz visibility update rate, selective probe updates for enabled, delta-encoded index buffer probe index buffer with caching, client view culling enabled.}
\label{fig:timeplot_nightstreet_culling}
\end{figure*}

\begin{figure*}[t]
\setlength\tabcolsep{2pt}%
\begin{tabularx}{\textwidth}{c}
   \includegraphics[ width=\linewidth, keepaspectratio]{figures/results_timeplots_latency_size/Latency_night_city_30_10_cache_no_cull.pdf}\\
   \includegraphics[ width=\linewidth, keepaspectratio]{figures/results_timeplots_latency_size/Size_night_city_30_10_cache_no_cull.pdf}\\
\end{tabularx}
\begin{tabularx}{\textwidth}{p{0.15\textwidth}p{0.25\textwidth}p{0.18\textwidth}p{0.20\textwidth}l}
\hline
Streaming Data & Average Latency (Std.Dev.) &  Min/Max Latency & Average Size (Std.Dev.) & Min/Max Size\\
\hline
Irradiance & 36.84 ms (18.258) & 16 ms / 274 ms & 3.82 kB (2.374) & 0.14 kB / 31.48 kB \\
Visibility & 31.97 ms (22.629) & 14 ms / 267 ms & 4.22 kB (4.044) & 0.15 kB / 35.46 kB \\
\hline
\end{tabularx}
\caption{\textbf{Detail time series plot for scene \textsc{Night Street} without view culling.}~\normalfont The scene is the same as in the previous plot with the difference that in this plot all changing probes are transferred to the client. The amount of streamed data is slightly higher than with client view culling enabled. However, our probe selection still significantly and consistently reduces the amount of streamed data with respect to the full probe volume containing 8000 probes. Streaming settings: 30 Hz irradiance update rate, 10 Hz visibility update rate, selective probe updates for enabled, delta-encoded index buffer probe index buffer with caching, client view culling disabled.}
\label{fig:timeplot_nightstreet_noculling}
\end{figure*}

\begin{figure*}[ht]
\centering
\includegraphics[width=0.65\textwidth]{figures/results_timeplots/bandwidth_nighstreet_w_uncompressed.pdf}
\caption{\textbf{Method overview showing consumed network bandwidth for scene \textsc{Night Street}.} The overview shows that our probe reduction and compression method reduce the required bandwidth between one and two orders of magnitude.}
\label{fig:bandwidthnightstreetwithuncompressed}
\end{figure*}

\begin{figure*}[ht]
\centering
\includegraphics[width=0.9\textwidth]{figures/results_timeplots/bandwidth_nighstreet_.pdf}
\caption{\textbf{Method overview (excluding uncompressed transfer) showing consumed network bandwidth for scene \textsc{Night Street}.}~\normalfont During recording the client moves on a fixed animation path through the scene. The consumed bandwidth is highest when the number of probes is high (0:07 to 0:12). 
Probe selection in combination with index caching optimizes for efficient temporal encoding of only changed probes resulting in a significant reduction of bandwidth compared to full volume encoding. Probe selection \textit{without} caching can actually increase the amount of transferred data as encoding efficiency is decreased.
Client view culling in combination with index caching helps to furthermore reduce the number of updated probes and maintain encoding efficiency.
As a result, culling and probe selection with index caching enable a significant reduction of bandwidth compared to full volume encoding.
}
\label{fig:bandwidthnightstreet}
\end{figure*}

%% %%%%%%%%%%%%%%%%%%%%%%%%%%%%%%%%%%%%%%%%%%%%%%%%%%%%%%%%%%%%%%%%%%%%%%%%%%%%%%%%%%%%%%%%%%%%%%%%%%%%%%%
% Tomb Buddha
%% %%%%%%%%%%%%%%%%%%%%%%%%%%%%%%%%%%%%%%%%%%%%%%%%%%%%%%%%%%%%%%%%%%%%%%%%%%%%%%%%%%%%%%%%%%%%%%%%%%%%%%%

\begin{figure*}[t]
\setlength\tabcolsep{2pt}%
\begin{tabularx}{\textwidth}{c}
   \includegraphics[ width=\linewidth, keepaspectratio]{figures/results_timeplots_latency_size/Latency_tomb_30-30_cache_cull_indirect.pdf}\\
   \includegraphics[ width=\linewidth, keepaspectratio]{figures/results_timeplots_latency_size/Size_tomb_30-30_cache_cull_indirect.pdf}\\
\end{tabularx}
\begin{tabularx}{\textwidth}{p{0.15\textwidth}p{0.25\textwidth}p{0.18\textwidth}p{0.20\textwidth}l}
\hline
Streaming Data & Average Latency (Std.Dev.) &  Min/Max Latency & Average Size (Std.Dev.) & Min/Max Size\\
\hline
Irradiance & 26.33  ms (18.295) & 15 ms / 174 ms & 1.64 kB (5.697) & 0.03 kB / 44.62 kB \\
Visibility & 30.63 ms (25.925) & 12 ms, Max 204 ms & 12.55 kB (56.536) & 0.04 kB / 419.89 kB \\
\hline
\end{tabularx}
\caption{\textbf{Detail time series plot for scene \textsc{Tomb Buddha} with view culling.}~\normalfont In this scene the client view includes almost all probes in the scene. Both lighting and visibility in the scene permanently change rapidly when the roof of the building caves in (time 0:18 to 0:35). This is the most challenging scenario for the streaming approach as all probe data must be transmitted resulting in a spike of consumed bandwidth and transfer latency. However, the perceived latency is still well under the perception threshold for diffuse GI latency (< 500 ms) [Crassin et al., CloudLight, 2015]. It is apparent that the costs for changing visibility of all probes in the volume dominate the costs for updating irradiance. Streaming settings: 30 Hz irradiance update rate, 30 Hz visibility update rate, selective probe updates for enabled, delta-encoded index buffer probe index buffer with caching, client view culling enabled.}
\label{fig:timeplot_tombbuddha_culling}
\end{figure*}

\begin{figure*}[t]
\setlength\tabcolsep{2pt}%
\begin{tabularx}{\textwidth}{c}
   \includegraphics[ width=\linewidth, keepaspectratio]{figures/results_timeplots_latency_size/Latency_tomb_30-10-30_cache_no_cull.pdf}\\
   \includegraphics[ width=\linewidth, keepaspectratio]{figures/results_timeplots_latency_size/Size_tomb_30-10-30_cache_no_cull.pdf}\\
\end{tabularx}
\begin{tabularx}{\textwidth}{p{0.15\textwidth}p{0.25\textwidth}p{0.18\textwidth}p{0.20\textwidth}l}
\hline
Streaming Data & Average Latency (Std.Dev.) &  Min/Max Latency & Average Size (Std.Dev.) & Min/Max Size\\
\hline
Irradiance & 26.21 ms (23.267) & 14 ms / 180 ms & 4.36 kB (9.829) & 0.03 kB / 55.97 kB \\
Visibility & 30.07 ms (32.731) & 13 ms / 238 ms & 26.41 kB (90.008) & 0.04  kB / 601.44 kB \\
\hline
\end{tabularx}
\caption{\textbf{Detail time series plot for scene \textsc{Tomb Buddha} without view culling.}~\normalfont Please see the explanation of the previous plot with the difference that in this plot all changing probes are transferred to the client. As in the previous plot the costs for changing visibility of all probes in the volume dominate the costs for updating irradiance. Streaming settings: 30 Hz irradiance update rate, 30 Hz visibility update rate, selective probe updates for enabled, delta-encoded index buffer probe index buffer with caching, client view culling disabled.}
\label{fig:timeplot_tombbuddha_noculling}
\end{figure*}

\begin{figure*}[ht]
\centering
\includegraphics[width=0.65\textwidth]{figures/results_timeplots/bandwidth_tomb_w_uncompressed.pdf}
\caption{\textbf{Method overview showing consumed network bandwidth for scene \textsc{Tomb Buddha}.} Our probe reduction and compression method reduce the required network traffic by one order of magnitude for this worst-case scenario scene.}
\label{fig:bandwidthtombwithuncompressed}
\end{figure*}

\begin{figure*}[ht]
\centering
\includegraphics[width=0.95\textwidth]{figures/results_timeplots/bandwidth_tomb_.pdf}
\caption{\textbf{Method overview (excluding uncompressed transfer) showing consumed network bandwidth for scene \textsc{Tomb Buddha}.}~\normalfont During recording the client moves on a fixed animation path through the scene. The consumed bandwidth is highest when the roof of the building in the scene is caving in (0:03 to 0:06) resulting in a change in visibility and irradiance for almost all probes. Probe selection in combination with index caching optimizes for efficient temporal encoding of only changed probes resulting in a significant reduction of bandwidth compared to full volume encoding. Probe selection without caching can actually increase the amount of transferred data as encoding efficiency is decreased. Client view culling in combination with index caching helps to furthermore reduce the number of updated probes and maintain encoding efficiency.}
\label{fig:bandwidthtomb}
\end{figure*}
